# Supplementary material for: Randomized Manifold Smoothing for Formal Robustness to Semantic Perturbations
Source: arXiv:2611.36126 source file (2026-11-26)
Supplement: Supplementary file 2 [file celeba_mani_radii_app.tex]

% ============================================================
% CSV FILE
% ============================================================

\newcommand{\celebaManiCertCSV}
{data/classification/celeba_mani_approx_certified_accuracy_table.csv}

% ============================================================
% NUMBER FORMAT
% ============================================================

\newcommand{\pct}[1]{%
    \fpeval{round(100*(#1),1)}%
}

\newcommand{\noisevalfmt}[1]{%
    \fpeval{round(#1,2)}%
}

% ============================================================
% TABLE
% ============================================================

\begin{table}[H]
\centering
\caption{
\textbf{Approximate Certified accuracy across whitened manifold radii on CelebA.}
For each smoothing scale $\sigma$, entries report the percentage of the
evaluation set that is correctly classified, non-abstaining, and certified
with whitened radius $r_{\mathrm{white}}$ at least the corresponding
threshold.
}
\label{tab:celeba_mani_radius}

\scriptsize
\setlength{\tabcolsep}{5pt}
\renewcommand{\arraystretch}{1.08}

\begin{tabular}{c c c c c c c c c c c c}
\toprule

\multirow{2}{*}{$\sigma$}
&
\multicolumn{11}{c}{\textbf{Manifold ($r_{\mathrm{white}}$)}}
\\

\cmidrule(lr){2-12}

$\noisevalma$
&
$0$
&
$0.1$
&
$0.25$
&
$0.5$
&
$0.75$
&
$1.0$
&
$1.25$
&
$1.5$
&
$2.0$
&
$2.5$
&
$3.0$
\\

\midrule

\csvreader[
filter test={
    \ifboolexpr{
        test {\ifdimcomp{\noiseval pt}{=}{0.02pt}}
        or
        test {\ifdimcomp{\noiseval pt}{=}{0.05pt}}
        or
        test {\ifdimcomp{\noiseval pt}{=}{0.10pt}}
        or
        test {\ifdimcomp{\noiseval pt}{=}{0.20pt}}
        or
        test {\ifdimcomp{\noiseval pt}{=}{0.50pt}}
        or
        test {\ifdimcomp{\noiseval pt}{=}{1.00pt}}
        or
        test {\ifdimcomp{\noiseval pt}{=}{2.00pt}}
    }
},
late after line=\\
]
{\celebaManiCertCSV}
{
sigma=\noiseval,
r_ge_0=\rzero,
r_ge_0.1=\rone,
r_ge_0.25=\rtwofive,
r_ge_0.5=\rfive,
r_ge_0.75=\rsevenfive,
r_ge_1=\ronezero,
r_ge_1.25=\roneTwoFive,
r_ge_1.5=\roneFive,
r_ge_2=\rtwo,
r_ge_2.5=\rtwoFive,
r_ge_3=\rthree
}
{%
\noisevalfmt{\noiseval}
&
\pct{\rzero}
&
\pct{\rone}
&
\pct{\rtwofive}
&
\pct{\rfive}
&
\pct{\rsevenfive}
&
\pct{\ronezero}
&
\pct{\roneTwoFive}
&
\pct{\roneFive}
&
\pct{\rtwo}
&
\pct{\rtwoFive}
&
\pct{\rthree}
}
\bottomrule
\end{tabular}

\end{table}
