# Supplementary material for: Randomized Manifold Smoothing for Formal Robustness to Semantic Perturbations
Source: arXiv:2611.36126 source file (2026-11-26)
Supplement: Supplementary file 3 [file full_certification_appendix_v1.tex]

\definecolor{gaincolor}{RGB}{55,160,75}

% Normal value
\newcommand{\plaincell}[1]{%
    \makebox[0pt][c]{#1}%
}

% Bold value + green gain.
% Gain does NOT affect alignment of the main value.
\newcommand{\gaincell}[2]{%
    \makebox[0pt][c]{%
        \textbf{#1}%
        \rlap{\hspace{0.15em}{\scriptsize\textcolor{gaincolor}{#2\%}}}%
    }%
}
\small
\begin{table}[t]
\centering
\caption{
Certification performance across representative tasks, datasets, and
representation spaces. Bold values indicate improved manifold-smoothing
performance, with green values reporting the corresponding improvement over
isotropic smoothing. $\uparrow$/$\downarrow$ indicate the preferred direction.
Full noise sweeps are reported in the Appendix \ref{app:..}.
}
\label{tab:main_certification}

\small
\setlength{\tabcolsep}{9pt}
\renewcommand{\arraystretch}{1.06}

\begin{tabular}{
@{}
c@{\hspace{13pt}}
c@{\hspace{13pt}}
l@{\hspace{13pt}}
c c c c c c
@{}
}
\toprule
\multirow[c]{2}{*}{\rotatebox[origin=c]{90}{Task}}
&
\multirow[c]{2}{*}{\rotatebox[origin=c]{90}{Dataset}}
&
\multirow[c]{2}{*}{Metric}
&
\multicolumn{6}{c}{Noise scale $\sigma$} \\

\cmidrule(lr){4-9}

& & &
0.02 & 0.05 & 0.07 & 0.10 & 0.50 & 1.00 \\
\midrule

% ============================================================
% Classification — CelebA
% ============================================================
\multirow{12}{*}{\rotatebox{90}{Classification}}
&
\multirow{6}{*}{\rotatebox{90}{CelebA}}
& Acc.$_{\mathrm{Iso}}$ $\uparrow$
    & \plaincell{93.0}
    & \plaincell{87.0}
    & \plaincell{84.0}
    & \plaincell{72.0}
    & \plaincell{45.0}
    & \plaincell{45.0} \\
&
& Acc.$_{\mathrm{Mani}}$ $\uparrow$
    & \plaincell{92.0}
    & \gaincell{92.0}{5.7}
    & \gaincell{92.0}{9.5}
    & \gaincell{92.0}{27.8}
    & \gaincell{92.0}{104.4}
    & \gaincell{86.0}{91.1} \\

&
& $\varnothing_{\mathrm{Iso}}$ $\downarrow$
    & \plaincell{0.0}
    & \plaincell{3.0}
    & \plaincell{2.0}
    & \plaincell{2.0}
    & \plaincell{0.0}
    & \plaincell{0.0} \\
&
& $\varnothing_{\mathrm{Mani}}$ $\downarrow$
    & \plaincell{0.0}
    & \gaincell{0.0}{100.0}
    & \gaincell{0.0}{100.0}
    & \gaincell{1.0}{50.0}
    & \plaincell{3.0}
    & \plaincell{11.0} \\

&
& $\log V_{\mathrm{Iso}}$
    & -2803.87 & -2345.73 & -2177.49 & -1999.16 & -1194.44 & -847.86 \\
&
& $\log V_{\mathrm{Mani}}$
    & -4107.49 & -3649.34 & -3481.11 & -3302.22 & -2497.44 & -2149.84 \\

\cmidrule(lr){2-9}

% ============================================================
% Classification — CelebA-HQ
% ============================================================
&
\multirow{6}{*}{\rotatebox{90}{CelebA-HQ}}
& Acc.$_{\mathrm{Iso}}$ $\uparrow$
    & \plaincell{\textbf{94.0}}
    & \plaincell{91.0}
    & \plaincell{85.0}
    & \plaincell{83.0}
    & \plaincell{50.0}
    & \plaincell{50.0} \\
&
& Acc.$_{\mathrm{Mani}}$ $\uparrow$
    & \plaincell{93.0}
    & \gaincell{92.0}{1.1}
    & \gaincell{92.0}{8.2}
    & \gaincell{92.0}{10.8}
    & \gaincell{93.0}{86.0}
    & \gaincell{86.0}{72.0} \\

&
& $\varnothing_{\mathrm{Iso}}$ $\downarrow$
    & 2.0 & 1.0 & 6.0 & 1.0 & 0.0 & 0.0 \\
&
& $\varnothing_{\mathrm{Mani}}$ $\downarrow$
    & 0.0 & 1.0 & 3.0 & 3.0 & 4.0 & 12.0 \\

&
& $\log V_{\mathrm{Iso}}$
    & -2803.87 & -2345.73 & -2177.49 & -1999.16 & -1194.44 & -847.86 \\
&
& $\log V_{\mathrm{Mani}}$
    & -4114.79 & -3656.91 & -3488.90 & -3310.57 & -2505.16 & -2157.54 \\

\midrule

% ============================================================
% Segmentation
% ============================================================
\multirow{6}{*}{\rotatebox{90}{Segmentation}}
&
\multirow{6}{*}{\rotatebox{90}{CelebAMask-HQ}}
& Acc.$_{\mathrm{Iso}}$ $\uparrow$
    & -- & -- & -- & 90.46 & 26.87 & 26.99 \\
&
& Acc.$_{\mathrm{Mani}}$ $\uparrow$
    & -- & -- & -- & \textbf{93.99} & \textbf{84.27} & \textbf{67.77} \\

&
& mIoU$_{\mathrm{Iso}}$ $\uparrow$
    & -- & -- & -- & 60.76 & 5.39 & 2.12 \\
&
& mIoU$_{\mathrm{Mani}}$ $\uparrow$
    & -- & -- & -- & \textbf{73.37} & \textbf{57.44} & \textbf{35.58} \\

&
& $\varnothing_{\mathrm{Iso}}$ $\downarrow$
    & -- & -- & -- & 5.87 & 40.07 & 8.81 \\
&
& $\varnothing_{\mathrm{Mani}}$ $\downarrow$
    & -- & -- & -- & 2.45 & 13.81 & 30.60 \\

\midrule

% ============================================================
% Concept Space
% ============================================================
\multirow{6}{*}{\rotatebox{90}{Concept Space}}
&
\multirow{6}{*}{\rotatebox{90}{ImageNet}}
& Acc.$_{\mathrm{Iso}}$ $\uparrow$
    & -- & -- & -- & 45.8 & 0.0 & 0.0 \\
&
& Acc.$_{\mathrm{Mani}}$ $\uparrow$
    & -- & -- & -- & \textbf{68.6} & \textbf{63.8} & \textbf{47.2} \\

&
& $\varnothing_{\mathrm{Iso}}$ $\downarrow$
    & -- & -- & -- & 48.0 & 100.0 & 100.0 \\
&
& $\varnothing_{\mathrm{Mani}}$ $\downarrow$
    & -- & -- & -- & 2.8 & 20.0 & 47.0 \\

&
& $\log V_{\mathrm{Iso}}$
    & -- & -- & -- & -1982.9 & -1184.0 & -840.0 \\
&
& $\log V_{\mathrm{Mani}}$
    & -- & -- & -- & -3220.7 & -2421.8 & -2077.8 \\

\bottomrule
\end{tabular}
\end{table}
